# Supplementary material for: Multi-Dimensional Optimization for Text Summarization via Reinforcement Learning
Source: arXiv:2406.00303 source file (2024-06-01)
Supplement: Supplementary file 3 [file fig-appendix-human.tex]

\begin{figure*}[!ht]
\centering
\includegraphics[width=0.85\textwidth]{fig/fig-appendix-human_p
.pdf}
\caption{}
\label{fig: appendix-human}
\end{figure*}

% \begin{figure*}[]
% \centering
% \includegraphics[width=0.93\textwidth]{fig/fig-appendix-chatgpt_ex2.pdf}
% \caption{}
% \label{fig: appendix-chatgpt_1}
% \end{figure*}
